# Supplementary material for: Mitigating Bias: Enhancing Image Classification by Improving Model Explanations
Source: arXiv:2307.01473 source file (2023-09-22)
Supplement: Supplementary file 1 [file appendix1.tex]

% \begin{figure}[htp]
% \begin{center}
% \includegraphics[width=1\textwidth]{vgg-visualization.png}
% \caption{Grad-CAM visualization results for images from RIVAL10 validation set using VGG16}\label{fig:visualization}
% \end{center}
% \end{figure}

% \begin{figure}[htp]
% \begin{center}
% \includegraphics[width=1\textwidth]{resnet18_visualization.png}
% \caption{Grad-CAM visualization results for images from RIVAL10 validation set using Resnet18}\label{fig:visualization}
% \end{center}
% \end{figure}

% \begin{figure}[htp]
% \begin{center}
% \includegraphics[width=1\textwidth]{resnet50_visualization.png}
% \caption{Grad-CAM visualization results for images from RIVAL10 validation set using Resnet50}\label{fig:visualization}
% \end{center}
% \end{figure}
